# Supplementary material for: Graph Partitioning With Limited Moves
Source: arXiv:2402.15485 source file (2024-02-23)
Supplement: Supplementary file 2 [file supplementary.tex]

% \documentclass[twoside]{article}
%
% \usepackage{aistats2024}
%
% \begin{document}
%\onecolumn
%\aistatstitle{
%Supplementary Materials}
{\Large\textbf{SUPPLEMENTARY MATERIALS}}
%\input{fptas}

%\input{k2}
%\input{bichriteria}

%\input{hardness}

%\section{OMITTED PROOFS AND TABLES}

% \begin{proofof}{Lemma \ref{lem:size}}
% For each $v\in L$, we have $1-{X}_v^{\ell_v}>1-\lambda$. Since ${X}$ is a feasible solution of LP~\ref{tab:maxmove-lp}, $r\ge\sum_{v\in L}(1-{X}_v^{\ell_v})$. So $r>(1-\lambda)|L|$, and $|L|< \frac{r}{1-\lambda}$.
% \end{proofof}

% \begin{proofof}{Lemma \ref{lem:helper2}}
% By the triangle inequality we have $\sum_{j\neq i}|X_u^j-X_v^j|\ge |\sum_{j\neq i} X_u^j-\sum_{j\neq i} X_v^j| =|(1-X_u^i)-(1-X_v^i)|$, where the last equality used $\sum_j X_u^j=\sum_j X_v^j=1$. Therefore, $d_X(u,v)=\frac{1}{2}(|X_u^i-X_v^i|+\sum_{j\neq i}|X_u^j-X_v^j|)\ge |X_u^i-X_v^i|$.
% \end{proofof}

% \begin{proofof}{Lemma \ref{lem:max1terminal}}
% Suppose there exists two distinct terminal nodes $s_i$ and $s_j$ in $H_\mathbf{z}$. By constraint (C5) of LP~\ref{tab:maxmove-lp}, we have $\bar{X}_{s_i}^i=1$ and $\bar{X}^i_{s_j}=0$, providing $|\bar{X}_{s_i}^i-\bar{X}^i_{s_j}|=1$. On the other hand, by Lemma \ref{lem:rounding1} we have $|\bar{X}_{s_i}^i-\bar{X}^i_{s_j}|<g<1$. This is a contradiction and there can be at most one terminal in $H_\mathbf{z}$.
% \end{proofof}

\input{experiments_supp}

%\end{document}
